# Supplementary material for: On legitimate mining of cryptocurrency in the browser - a feasibility study
Source: arXiv:1812.04054 source file (2019-01-04)
Supplement: Supplementary file 1 [file appendix.tex]

\subsection{Definitions} \label{appendix_definitions}
\begin{itemize}
    \item \(M\): \hspace{1em} \= the amount of Monero coins earned in total;
    \item \(M_{usd}\): \hspace{1em} \= the US dollar value of 1 Monero on 17th of April, 2018;
    \item \(H\): \hspace{1em} \= the number of total hashes solved;
    \item \(D\): \hspace{1em} \= the global Monero mining difficulty on 17th of April, 2018;
    \item \(B\): \hspace{1em} \= the amount of Monero coins rewarded for a mined block on 17th of April, 2018;
    \item \(X_{c}\): \hspace{1em} \= the earnable share per coin with the pool fee deducted \cite{coinhive_pay_calc};
    \item \(R_{crypto}\): \hspace{1em} \= the revenue generated from mining cryptocurrency in US dollars;
    \item \(P_{rpm}\): \hspace{1em} \= net publisher revenue in US dollars;
    \item \(CPM_{avg}\): \hspace{1em} \= average CPM value \cite{cpm_average};
    \item \(X_{a}\): \hspace{1em} \= the charge applied by the advertisement network \cite{cpm_average};
    \item \(I\): \hspace{1em} \= total number of advertisement impressions;
    \item \(R_{ads}\): \hspace{1em} \= advertisement revenue in US dollars;
    \item \(A_{avg}\): \hspace{1em} \= average number of advertisement impressions per person;
    \item \(U_{avg}\): \hspace{1em} \= average hash rate of a single participant;
    \item \(T_{max}\): \hspace{1em} \= total session time of participants who selected mining;
    \item \(T_{avg}\): \hspace{1em} \= average session time of participants who selected mining;
    \item \(H_{max}\): \hspace{1em} \= maximum  number  of hashes if all participants were to select cryptocurrency mining;
    \item \(N\): \hspace{1em} \= total number of participants;
    \item \(R_{cryptoMax}\): \hspace{1em} \= maximum browser mining revenue;
    \item \(R_{adsMax}\): \hspace{1em} \= maximum potential advertisement revenue.
\end{itemize}
